# Supplementary material for: Mixed-Type Relational Database Synthesis with Graph-Prompted Language Model
Source: arXiv:2611.02373 source file (2026-11-02)
Supplement: Supplementary file 1 [file appendix.tex]

\subsection{Metric Definitions}
\label{app:metric_definitions}

Let $\mathcal{D}^{r}=\{T^{r}_{1},\ldots,T^{r}_{M}\}$ and
$\mathcal{D}^{s}=\{T^{s}_{1},\ldots,T^{s}_{M}\}$ denote the real
and synthetic databases, respectively.

\noindent\textbf{C2ST-Agg.}
C2ST-Agg measures whether real and synthetic records remain distinguishable after incorporating relational context. For each eligible table, we augment its records with features aggregated from related tables, including child counts, categorical cardinalities, and numerical means. A classifier is then trained to distinguish real from synthetic records. We report the mean classification accuracy across eligible tables, with values closer to random guessing indicating higher fidelity.

\noindent\textbf{Intra-table similarity.}
Intra-table similarity measures how well the synthetic database preserves dependencies between column pairs within individual tables. We compute a similarity score for each valid column pair and average the scores across all tables. Numerical and categorical attributes are compared using correlation- and contingency-based similarities, respectively. For pairs involving textual attributes, we use semantic embeddings to compare their dependency structures. Higher values indicate better preservation of pairwise relationships between attributes within the same table.

\noindent\textbf{Inter-table similarity.}
Inter-table similarity measures whether dependencies between attributes in directly related tables are preserved. For each parent--child relationship, we join the two tables through their primary- and foreign-key columns and evaluate similarities between cross-table column pairs. Text attributes are evaluated through their semantic representations. The final score averages all valid cross-table pairs, with higher values indicating better preservation of relational dependencies.

\noindent\textbf{Constraint violation rate.}
Following prior work~\cite{stoian2024realistic,zhao2026constraintaware}, we define CVR as the proportion of records identified as violating at least one reference semantic dependency. For a synthetic database, it is computed as
\[
\mathrm{CVR}(\mathcal{D}^{s})
=
\frac{
\sum_{m=1}^{M}
\sum_{i=1}^{|T^{s}_{m}|}
\mathbb{I}\!\left[
T^{s}_{m,i}
\text{ violates a dependency in }\mathcal{C}
\right]
}{
\sum_{m=1}^{M}|T^{s}_{m}|
}.
\]
A record that violates multiple dependencies is counted only once. For cross-table, group-level, and temporal dependencies, violations are attributed to the corresponding records involved in the violation. Lower values indicate better semantic consistency, and $\mathrm{CVR}=0$ means that no violation is detected under the evaluated reference dependency set.

\noindent\textbf{Utility.}
We evaluate downstream utility using the train-on-synthetic-test-on-real protocol. A relational prediction model is trained on each synthetic database and evaluated on the corresponding real test set. We report AUC for classification tasks and MAE for regression tasks. Higher AUC and lower MAE indicate that the synthetic database better preserves task-relevant information.

\subsection{Reference Semantic Dependency Sets}
\label{app:reference_constraints}

We construct a dataset-specific reference semantic dependency set through repeated LLM-assisted dependency elicitation and human verification. For each dataset, the LLM independently proposes candidate dependencies over multiple runs using the database schema, column descriptions, and sampled records. This repeated procedure broadens dependency coverage and reduces reliance on a single LLM response.

Human reviewers subsequently consolidate semantically equivalent proposals and verify each candidate against the database schema, the complete real database, and the intended semantics of the involved attributes and relationships. We retain only dependencies that are semantically valid, supported by the reference data, and practically meaningful for assessing database synthesis. We discard accidental correlations, dataset-specific identifier mappings, redundant dependencies, and rules without a clear semantic interpretation. The resulting reference sets are frozen before evaluating synthetic databases.

The retained dependencies cover intra-table attribute dependencies, primary- and foreign-key relationships, cross-table consistency, temporal ordering, aggregation relationships, and domain-specific validity rules. The complete dependency definitions, their applicable tables and attributes, and their validation evidence are reported in the following dataset-specific tables. The same reference set is used for the text-free and text-rich versions of a dataset when their relational schemas and structured attributes are unchanged.

\subsection{Implementation and Settings of GReaT-Based Baselines}
\label{app:great_baselines}

\subsubsection{GReaT-Cond}
\label{app:great_cond}

\subsubsection{GReaT-Join}
\label{app:great_join}

\subsection{Additional Experimental Results}
\label{app:additional_results}

\subsubsection{Efficiency Comparison}
\label{app:efficiency}

\begin{table*}[t]
\centering
\caption{Efficiency comparison. Training time, generation time, and total time are measured in minutes.}
\label{tab:app_efficiency_comparison}
\resizebox{\textwidth}{!}{%
\renewcommand{\arraystretch}{0.82}%
\setlength{\aboverulesep}{0.15ex}%
\setlength{\belowrulesep}{0.15ex}%
\begin{tabular}{@{}llccccccc@{}}
\toprule
Dataset & Metric & SDV & RC-TGAN & RelDiff & GRDM & TabARGN & REaLTabF. & \our \\
\midrule
\multirow{3}{*}{Walmart}
& Train ($\downarrow$) & 0.07 & 26.05 & 26.97 & 1089.82 & 1.39 & 56.50 & 106.72 \\
& Generate ($\downarrow$) & 0.14 & 0.01 & 0.60 & 29.32 & 0.02 & 0.23 & 2.62 \\
& Total ($\downarrow$) & 0.21 & 26.06 & 27.57 & 1119.18 & 1.42 & 56.73 & 109.34 \\
\addlinespace[3pt]
\multirow{3}{*}{Biodeg.}
& Train ($\downarrow$) & 3.23 & 34.10 & 94.90 & 1022.40 & 0.23 & \NA & 47.12 \\
& Generate ($\downarrow$) & 14.63 & 0.03 & 1.08 & 70.40 & 0.01 & \NA & 0.78 \\
& Total ($\downarrow$) & 17.86 & 34.13 & 95.98 & 1092.80 & 0.24 & \NA & 47.90 \\
\addlinespace[3pt]
\multirow{3}{*}{\shortstack[l]{F1\\(w.o.\ text)}}
& Train ($\downarrow$) & 14.61 & 146.76 & 815.80 & 1374.76 & 5.52 & \NA & 278.84 \\
& Generate ($\downarrow$) & 21.92 & 0.07 & 7.48 & 457.47 & 0.06 & \NA & 27.93 \\
& Total ($\downarrow$) & 36.53 & 146.83 & 823.28 & 1832.60 & 5.58 & \NA & 306.77 \\
\addlinespace[3pt]
\multirow{3}{*}{\shortstack[l]{F1\\(w.\ text)}}
& Train ($\downarrow$) & \NA & \NA & \NA & \NA & 6.47 & \NA & 257.73 \\
& Generate ($\downarrow$) & \NA & \NA & \NA & \NA & 0.13 & \NA & 24.42 \\
& Total ($\downarrow$) & \NA & \NA & \NA & \NA & 6.60 & \NA & 282.15 \\
\addlinespace[3pt]
\multirow{3}{*}{Chicago}
& Train ($\downarrow$) & \NA & \NA & \NA & \NA & 5.72 & \NA & 104.75 \\
& Generate ($\downarrow$) & \NA & \NA & \NA & \NA & 0.06 & \NA & 40.57 \\
& Total ($\downarrow$) & \NA & \NA & \NA & \NA & 5.78 & \NA & 145.32 \\
\addlinespace[3pt]
\multirow{3}{*}{ML100K}
& Train ($\downarrow$) & \NA & \NA & \NA & \NA & 4.60 & \NA & 129.72 \\
& Generate ($\downarrow$) & \NA & \NA & \NA & \NA & 0.05 & \NA & 28.82 \\
& Total ($\downarrow$) & \NA & \NA & \NA & \NA & 4.65 & \NA & 158.54 \\
\bottomrule
\end{tabular}
}
\end{table*}


\subsubsection{Semantic Dependency Engine Analysis}
\label{app:constraint_engine}

\begin{table*}[t]
\centering
\caption{Semantic dependency analysis. We report the constraint violation rate (CVR, $\downarrow$) across datasets. The ablation row evaluates the necessity of the semantic dependency engine, while the LLM rows evaluate the sensitivity of dependency discovery and program generation to the LLM used by the semantic dependency engine. $^\star$\,Default configuration used in the main experiments.}
\label{tab:app_constraint_cvr}
\resizebox{\textwidth}{!}{%
\renewcommand{\arraystretch}{0.82}%
\setlength{\aboverulesep}{0.15ex}%
\setlength{\belowrulesep}{0.15ex}%
\begin{tabular}{@{}llccccccc@{}}
\toprule
Analysis & Setting
  & Walmart & Biodeg.
  & F1 (w.o.\ text) & F1 (w.\ text)
  & Chicago & ML100K
  & Avg.\,CVR ($\downarrow$) \\
\midrule
\multirow{2}{*}{Ablation}
 & \our                  & 0 & 0 & 0 & 0 & 0 & 0 & 0 \\
 & w/o Semantic Dependency Engine  & \NA & \NA & \NA & \NA & \NA & \NA & \NA \\
\addlinespace[3pt]
\multirow{3}{*}{Semantic Dependency Engine LLM}
 & GPT-5.5$^\star$        & 0 & 0 & 0 & 0 & 0 & 0 & 0 \\
 & DeepSeek-v4-pro        & \NA & \NA & \NA & \NA & \NA & \NA & \NA \\
 & Claude Sonnet-4.6      & \NA & \NA & \NA & \NA & \NA & \NA & \NA \\
\bottomrule
\end{tabular}
}
\end{table*}


\subsubsection{Hyperparameter Sensitivity}
\label{app:hyperparameters}

\begin{table*}[t]
\centering
\caption{Hyperparameter sensitivity analysis. We report C2ST-Agg ($\downarrow$, \%) averaged over three runs. $^\star$\,Default configuration used in the main experiments.}
\label{tab:app_hyperparameters}
\resizebox{\textwidth}{!}{%
\renewcommand{\arraystretch}{0.82}%
\setlength{\aboverulesep}{0.15ex}%
\setlength{\belowrulesep}{0.15ex}%
\begin{tabular}{@{}llccccccc@{}}
\toprule
Hyperparameter & Setting
  & Walmart & Biodeg.
  & F1$^{-\text{T}}$ & F1$^{+\text{T}}$
  & Chicago & ML100K
  & Avg.\,($\downarrow$) \\
\midrule
\multirow{3}{*}{Decode LLM}
 & Qwen3-0.6B$^\star$     & 62.96 & 57.29 & 65.53 & 74.36 & 73.89 & 78.02 & 68.68 \\
 & Qwen3-1.7B             & 47.78 & 57.08 & 68.97 & 84.77 & 87.42 & 84.20 & 71.70 \\
 & Qwen3-4B               & 64.44 & 58.85 & 63.63 & 76.58 & 80.18 & 75.20 & 69.81 \\
\addlinespace[3pt]
\multirow{3}{*}{Res.\ Dropout}
 & 0.2                    & 46.67 & 56.22 & 63.78 & 74.54 & 76.57 & 76.69 & 65.75 \\
 & 0.4$^\star$            & 62.96 & 57.29 & 65.53 & 74.36 & 73.89 & 78.02 & 68.68 \\
 & 0.6                    & 62.22 & 57.65 & 69.76 & 80.22 & 77.69 & 81.86 & 71.57 \\
\addlinespace[3pt]
\multirow{3}{*}{Decode Temp.}
 & 0.6                    & 52.22 & 57.30 & 67.21 & 75.43 & 73.61 & 82.41 & 68.03 \\
 & 0.8$^\star$            & 62.96 & 57.29 & 65.53 & 74.36 & 73.89 & 78.02 & 68.68 \\
 & 1.0                    & 60.00 & 56.39 & 62.68 & 75.05 & 76.72 & 73.40 & 67.37 \\
\addlinespace[3pt]
\multirow{3}{*}{Num Soft Prompt Token}
 & 1                      & 62.96 & 57.29 & 65.53 & 74.36 & 73.89 & 78.02 & 68.68 \\
 & 2                      & 52.22 & 56.32 & 62.41 & 80.69 & 77.43 & 78.20 & 69.55 \\
 & 4                      & 53.33 & 57.37 & 64.45 & 76.07 & 73.16 & 77.18 & 66.93 \\
\bottomrule
\end{tabular}
}
\end{table*}
